# Supplementary material for: Efficacy of Bayesian Neural Networks in Active Learning
Source: arXiv:2104.00896 source file (2021-04-19)
Supplement: Supplementary file 1 [file supplementary.tex]

\section{Appendix}
\subsection{Model Settings}
\label{appendix:a}

The details of training,  testing,  and architecture of models used in this paper are explained below.

\noindent {\bf Train and test procedure } During training 5\% of data is allotted for evaluation.  For both continual training and retraining from scratch,  the training is stopped if there is no performance improvement on the validation dataset for $20$ epochs.  During testing,  we create ensembles of five trained models and evaluate each instance on the test data. The results (i.e., accuracy,  precision, etc) from each ensemble  is averaged to get the final output.   

%Note that for EN,  each independently trained network already forms the ensemble, 
%Since BNN,  MCD and EN have differences in the form of regularization,  where in MCDs are regularized using dropouts,  BNN using KL,  it is difficult to obtain the exact same accuracy after the first training round (i.e., on the seed set). To overcome this issue, we set a very large epoch number and use an early stopping criteria. 

\noindent {\bf Neural network architectures}: Four different neural network architectures are used in this paper. For CNNs, the architecture comprises of two segments (a) \textit{feature selection network}, which consists of convolution layer combined with maxpool layer and (b) a \textit{classifier network}, which consists of some densely connected layers. For all CNN models, the classifier network has two dense layers with $512 \rightarrow256 \rightarrow10$ parameters, where $\rightarrow$ indicates the flow (or direction) of layers and the neurons in the last layer correspond to the number of class labels.  For regression, the last layer has just one neuron. The architectures are explained as follows:
\begin{enumerate}[(a)]
\itemsep0em
	\item {\bf LeNetD2}: A simple 2 layer NN with $300 \rightarrow 100$ neurons. For MCD, dropouts are applied to the intermediate layer (set as 0.5). For EN and BNN no dropouts are applied.
	\item {\bf LeNet5 \cite{lecun1998gradient}} : This classic architecture consists of 2 CNN layers with filter sizes $6\rightarrow16$ followed by a classifier network. Between each CNN, we add a maxpool layer where the kernel size and stride are set as two.
	\item {\bf AlexNet Light}: This is a simplified version of the Alexnet architecture that is similar to the four layer CNN implemented in Keras library \footnote{https://github.com/keras-team/keras}. Here, we have four CNN layers with filters $32\rightarrow32\rightarrow64\rightarrow64$ followed by the classifier network. The setting for maxpool layer is as follows: kernel size=3, stride=1, padding=1 for the first CNN layer and padding=0 and stride=1 for subsequent CNN layers.
	\item {\bf VGG}: There are several variations of VGG \cite{simonyan2014very}. For our experiments we use VGG19 with 16 CNN layers $64(2)\rightarrow128(2)\rightarrow256(4)\rightarrow512(4)\rightarrow512(4)$, where (x) indicates the number of filters, for instance, 64(2) implies $64\rightarrow64$. As with other CNNs, the feature selection network is followed by the classifier network. The kernel size and stride of maxpool are set as two.
	\item {\bf Densenet}: We use Densenet121, which has 5 convolution layers, 3 transition layers, 1 classification layer and 2 dense block as introduced in  \cite{huang2017densely}.
\end{enumerate}

\noindent {\bf Parameter setting}: The weights of all layers are initialized with Kaiming uniform distribution \footnote{www.pytorch.org/docs/stable/nn.init.html}. Adam \footnote{www.pytorch.org/docs/stable/optim.html} is used as the optimization algorithm of choice.  The batch size is set to $32$ for smaller models such as LeNetD2, LeNet5 and AlexNet Light, for VGG and Densenet,  it is set to $256$.  
The model-specific details and hyper-parameter setting is explained as follows: 
\begin{itemize}
	\item {\bf BNN}: The KL scaling factor is set as $1/N_r$ where $N_r$ is the number of samples per round. The mean of the network parameters $\mathbf{w}$ is set as $\mathcal{N}(0,  \sigma)$. Here, $\sigma = 1/\sqrt{\mathbf{w}^{\ell}_{n}}$, where $\mathbf{w}^{\ell}_{n}$ is the input dimension of $\mathbf{w}$ in $\ell^{\text{th}}$ layer.  The variance of $\mathbf{w}$ is sampled from $\mathcal{N}(-9, 10^{-3})$.  The mean and variance of prior $\mathbf{z}$ is sampled from  $\mathcal{N}(1,  10^{-3})$ and $\mathcal{N}(-9, 10^{-3})$ respectively.
	\item {\bf MCD}: In MCD, the dropouts are activated during two phases (a) training and (b) \textit{active learning} . During testing, the dropouts are turned off. For all dense layers, the dropout is set as 0.5 and for convolution layers, it is set to 0.25.
\end{itemize}
